# Supplementary material for: Prompt to Polyp: Medical Text-Conditioned Image Synthesis with Diffusion Models
Source: arXiv:2505.05573 source file (2025-05-12)
Supplement: Supplementary file 1 [file appendix.tex]

\section*{Appendix}

\appendix
